# Supplementary material for: Contextual Moral Value Alignment Through Context-Based Aggregation
Source: arXiv:2403.12805 source file (2024-03-19)
Supplement: Supplementary file 1 [file suplements.tex]

\section{alternative definition}
\subsection{Multi-Moral Value alignment}
A (large) language model (LLM) is a parametric probability distribution $p_w(y)$ over sequence of tokens $Y=(y_1,\ldots,y_m)$, with $w$ the LLM parameter weights. Given a LLM of weights $w$, we can generate new token from it by sampling from $y \sim p_w(\,\cdot\,|x)$.

We define the value alignment $AL(LLM_{\alpha},LLM_{\beta})$ between two text generation model \(LLM_{\alpha}\) and \(LLM_{\beta}\) as

\begin{align*}
AL(LLM_{\alpha},LLM_{\beta})= \frac{1}{|x|}\sum_{x} E(V(Y^{x}_{\alpha}),V(Y^{x}_{\beta}))
\end{align*}

Where, \(Y_{\alpha}\) and \(Y_{\beta}\) are the tokens generated by \(LLM_{\alpha}\) and \(LLM_{\beta}\) respectively.

- $E$ is a similarity metric to measure the similarity between \(V(Y_{\alpha})\) and \(V(Y_{\beta})\).

- \(V(Y_{\alpha})\) and \(V(Y_{\beta})\) are vectors representing the moral alignment of \(Y_{\alpha}\) and \(Y_{\beta}\) respectively across different moral values:
      \[ V(Y_{\alpha}) = [cl_{1}^{\alpha}, cl_{2}^{\alpha}, \ldots, cl_{n}^{\alpha}] \]
      \[ V(Y_{\beta}) = [cl_{1}^{\beta}, cl_{2}^{\beta}, \ldots, cl_{n}^{\beta}] \]
      
- \(cl_{i}^{\alpha}\) and \(cl_{i}^{2}\) are the classifications for \(Y_{\alpha}\) and \(Y_{2}\) based on moral value \(i\), obtained from multiple classifiers.

\subsection{Contextual Multi-values alignment:}
The goal is to align the model’s behavior across various contexts. In this case, alignment refers to the model producing outputs that are consistent
with specified values or objectives. The alignment problem involves finding a set of parameters for the model such that it meets the desired criteria
across a range of contexts.

\begin{align*}
AL(LLM_{\alpha},LLM_{\beta})= \frac{1}{|C|} \frac{1}{|x|}\sum_{C}\sum_{x} E(V_C(Y^{x}_{\alpha}),V_C(Y^{x}_{\beta}))
\end{align*}

where \[ V_C(Y_{\alpha}) \] is the vector representing the moral alignment following the context $C$.

We model Contextual multi-value alignment as a contextual multi-objective reinforcement learning problem involves finding a policy that optimally balances multiple objectives simultaneously, aligning the agent's actions with a set of desired values while taking into account the context. The context in our setting would be the moral value 

Let $\mathcal{S}$ be the state space, $\mathcal{A}$ be the action space, $\mathcal{C}$ be the context space, and $\mathcal{R} \subseteq \mathbb{R}^N$ be the set of possible rewards, where $N$ is the number of objectives.

A contextual multi-value alignment problem in the context of contextual multi-objective reinforcement learning (CMORL) is defined by a tuple $\langle \mathcal{S}, \mathcal{A}, \mathcal{C}, \mathcal{P}, \mathcal{R}, \gamma \rangle$, where:
\begin{itemize}
    \item $\mathcal{P}: \mathcal{S} \times \mathcal{C} \times \mathcal{A} \times \mathcal{S} \rightarrow [0, 1]$ is the transition probability function representing the dynamics of the environment with respect to the context which is in this setting the .
    \item $\mathcal{R}(s, c, a, s') \in \mathcal{R}$ is the reward function that maps state-context-action-state transitions to a vector of rewards, where $\mathcal{R}(s, c, a, s') = \langle r_1, r_2, \ldots, r_N \rangle$ with each $r_i$ representing the reward for the $i$th moral value.
    \item $\gamma$ is the discount factor, $0 \leq \gamma \leq 1$, which weighs future rewards.
\end{itemize}

Given a policy $\pi: \mathcal{S} \times \mathcal{C} \rightarrow \mathcal{P}(\mathcal{A})$, where $\mathcal{P}(\mathcal{A})$ is the set of probability distributions over actions, the objective in contextual multi-value alignment CMORL is to find a policy that maximizes or minimizes the rewards for each objective simultaneously while considering the context.

Formally, we seek a policy $\pi^*$ that maximizes the vector-valued performance measure $\mathbf{J}(\pi)$, where $\mathbf{J}(\pi) = \langle J_1(\pi), J_2(\pi), \ldots, J_N(\pi) \rangle$ and $J_i(\pi)$ represents the expected return with respect to the $i$th objective, given the context.

\[
\pi^* = \arg \max_{\pi} \mathbf{J}(\pi) \top c_t
\]

Where $c_t$ is the Moral Profile is typically refers to a representation of an individual's moral values, beliefs, or preferences in a structured form of a vector. This vector might encode different dimensions or aspects of moral considerations.

For instance, if we consider a simplified example where moral values are represented along several dimensions (e.g., fairness, honesty, compassion), a Moral Profile Vector for an individual is described as:
\begin{eqnarray*}
 c_t = [i_1, i_2, i_3, \ldots, i_n] 
\end{eqnarray*}
Here, \( i_1, i_2, i_3, \ldots, i_n \) are values representing the degree to which the individual adheres to or prioritizes certain moral principles or values.
